# Supplementary material for: The Limits of Differential Privacy in Online Learning
Source: arXiv:2411.05483 source file (2025-03-17)
Supplement: Supplementary file 1 [file impact.tex]

\section{Broader Impacts}
\label{sec:impact}

Privacy has become a fundamental concern in today's machine learning community. In this work, we show several lower bounds and upper bounds on private online learning tasks. While our contributions are theoretical in nature, and we do not see any direct societal implications, we hope that our results will reveal the intrinsic structures of the problems and provide insights for the development of practical online learning algorithms with better privacy-utility trade-offs.
